# Supplementary material for: Shortcut to geostrophy in wave-driven rotating turbulence: the quartetic instability
Source: arXiv:2003.01177 ancillary file (2020-03-02)
Supplement: Supplementary file 1 [file 2020_brunet_prl_SM.pdf]

# —Supplemental Material—
# Shortcut to geostrophy in wave-driven rotating turbulence: the quartetic instability

Maxime Brunet,[1] Basile Gallet,[2] and Pierre-Philippe Cortet[1]

[1]*Laboratoire FAST, CNRS, Université Paris-Sud, Université Paris-Saclay, 91405 Orsay, France*
[2]*Service de Physique de l'État Condensé, CEA Saclay, CNRS, Université Paris-Saclay, 91191 Gif-sur-Yvette, France*

We detail here the precise conventions considered throughout the Letter, and the asymptotic expansions leading to the quartetic evolution equations and to the quartetic interaction coefficients. Following Smith & Waleffe [1], we decompose the velocity field onto the wavevectors of a triply periodic box, using a helical basis:

$$\mathbf{u} = \Sigma_{\mathbf{k}} \Sigma_{s=\pm 1} b_s(\mathbf{k}, t) \mathbf{h}_s(\mathbf{k})\, e^{i[\mathbf{k}\cdot\mathbf{x} - \omega_s(\mathbf{k}) t]}\,, \tag{1}$$

where the first sum is over all wavevectors $\mathbf{k}$. The helical basis vectors $\mathbf{h}_s(\mathbf{k})$ are defined as:

$$\mathbf{h}_s(\mathbf{k}) = \hat{\mathbf{k}} \times \frac{\mathbf{k}\times\hat{\mathbf{z}}}{|\mathbf{k}\times\hat{\mathbf{z}}|} + i\, s \frac{\mathbf{k}\times\hat{\mathbf{z}}}{|\mathbf{k}\times\hat{\mathbf{z}}|}\,, \tag{2}$$

where $\hat{\mathbf{z}}$ is the unit vector in the vertical direction, and $\hat{\mathbf{k}} = \mathbf{k}/|\mathbf{k}|$. The reality constraint for the velocity field imposes $b_s(\mathbf{k}, t) = \bar{b}_s(-\mathbf{k}, t)$. The helical basis vectors correspond to the spatial structure of inertial-wave modes, the frequency $\omega_s(\mathbf{k})$ of the mode at wavenumber $\mathbf{k}$ with polarity $s$ being given by the dispersion relation:

$$\omega_s(\mathbf{k}) = 2\Omega\, s\, \frac{\mathbf{k}\cdot\hat{\mathbf{z}}}{k}\,, \tag{3}$$

where $k = |\mathbf{k}|$.

## I. QUARTETIC INTERACTION COEFFICIENTS

Inserting the decomposition (1) into the rotating Navier-Stokes equation leads to:

$$(\partial_t + \nu k^2 + \mu\, \delta_{\mathbf{k}\cdot\hat{\mathbf{z}};0}) b_{s_\mathbf{k}} = \frac{1}{2}\sum C^{s_\mathbf{k} s_\mathbf{p} s_\mathbf{q}}_{\mathbf{kpq}} \bar{b}_{s_\mathbf{p}} \bar{b}_{s_\mathbf{q}} e^{i(\omega_{s_\mathbf{k}} + \omega_{s_\mathbf{p}} + \omega_{s_\mathbf{q}})t}\,. \tag{4}$$

This is equation (5) of SW, where we have included an additional $\mu$-term mimicking bottom drag acting on the 2D modes, using a kroenecker delta. The sum is over all wavenumbers $\mathbf{p}$ and $\mathbf{q}$ such that $\mathbf{k}+\mathbf{p}+\mathbf{q} = 0$, and over the polarities $s_\mathbf{p} = \pm 1$, $s_\mathbf{q} = \pm 1$. The triadic interaction coefficients are:

$$C^{s_\mathbf{k} s_\mathbf{p} s_\mathbf{q}}_{\mathbf{kpq}} = \frac{s_q q - s_p p}{2} [\bar{\mathbf{h}}_{s_p}(\mathbf{p}) \times \bar{\mathbf{h}}_{s_q}(\mathbf{q})] \cdot \bar{\mathbf{h}}_{s_k}(\mathbf{k})\,. \tag{5}$$

We non-dimensionalize Eq. (4) using the timescale $\Omega^{-1}$ and a length scale $L$ (for instance, the height of the fluid layer):

$$(\partial_{\tilde{t}} + \tilde{\nu}\tilde{k}^2 + \tilde{\mu}\, \delta_{\mathbf{k}\cdot\hat{\mathbf{z}};0}) \tilde{b}_{s_{\tilde{\mathbf{k}}}} = \frac{1}{2}\sum C^{s_\mathbf{k} s_\mathbf{p} s_\mathbf{q}}_{\tilde{\mathbf{k}}\tilde{\mathbf{p}}\tilde{\mathbf{q}}} \tilde{\bar{b}}_{s_\mathbf{p}} \tilde{\bar{b}}_{s_\mathbf{q}} e^{i(\tilde{\omega}_{s_\mathbf{k}} + \tilde{\omega}_{s_\mathbf{p}} + \tilde{\omega}_{s_\mathbf{q}})\tilde{t}}\,, \tag{6}$$

where $\tilde{t} = \Omega t$, $\tilde{\mathbf{k}} = \mathbf{k}L$, $\tilde{\nu} = \nu/L^2\Omega$, $\tilde{\mu} = \mu/\Omega$, $\tilde{b}_{s_{\tilde{\mathbf{k}}}} = b_{s_\mathbf{k}}/L\Omega$, $\tilde{\omega}_{s_{\tilde{\mathbf{k}}}} = \omega_{s_\mathbf{k}}/\Omega$. We drop the tildes in the following to alleviate notations. For rapid global rotation, the Rossby number based on the rms velocity $U$ is small, $Ro = U/L\Omega \ll 1$. We introduce a multiple timescale expansion:

$$b_{s_\mathbf{k}} = Ro\, b^{(0)}_{s_\mathbf{k}}(t, T_1, T_2) + Ro^2 b^{(1)}_{s_\mathbf{k}}(t, T_1, T_2) + Ro^3 b^{(2)}_{s_\mathbf{k}}(t, T_1, T_2) + \dots\,, \tag{7}$$

where the slow time variables are $T_1 = Ro\, t$ and $T_2 = Ro^2\, t$. We also consider the weakly damped regime, $\nu = Ro^2\, \nu_0$ and $\mu = Ro^2\, \mu_0$. In these relations, the quantities $\nu_0$, $\mu_0$, $b^{(0)}_{s_\mathbf{k}}(t, T_1, T_2)$, $b^{(1)}_{s_\mathbf{k}}(t, T_1, T_2)$ are at most of the order $\mathcal{O}(1)$. Inserting into Eq. (6) and collecting terms at order $\mathcal{O}(Ro)$ yields simply:

$$\partial_t b^{(0)}_{s_\mathbf{k}}(t, T_1, T_2) = 0\,, \tag{8}$$

i.e., the wave amplitudes do not vary on the fast timescale.

To order $\mathcal{O}(Ro^2)$, Eq. (6) yields:

$$\partial_t b^{(1)}_{s_{\mathbf{k}}} + \partial_{T_1} b^{(0)}_{s_{\mathbf{k}}} = \frac{1}{2}\sum C^{s_{\mathbf{k}} s_{\mathbf{p}} s_{\mathbf{q}}}_{\mathbf{kpq}}\, \bar{b}^{(0)}_{s_{\mathbf{p}}}\, \bar{b}^{(0)}_{s_{\mathbf{q}}}\, e^{i(\omega_{s_{\mathbf{k}}}+\omega_{s_{\mathbf{p}}}+\omega_{s_{\mathbf{q}}})t} \,. \tag{9}$$

Averaging the right-hand side with respect to the fast variable $t$ gives zero, except for resonant triads: if $\omega_{s_{\mathbf{k}}} + \omega_{s_{\mathbf{p}}} + \omega_{s_{\mathbf{q}}} = 0$, then the fast-time average is non-zero. When this is the case, we obtain $\partial_{T_1} b^{(0)}_{s_{\mathbf{k}}} \neq 0$ when averaging (9): this evolution with time $T_1$ corresponds to the standard nonlinear interactions within resonant triads of waves. Upon subtracting the $t$-average of (9) from the full Eq. (9), we obtain:

$$\partial_t b^{(1)}_{s_{\mathbf{k}}} = \frac{1}{2} \sum_{\omega_{s_{\mathbf{k}}}+\omega_{s_{\mathbf{p}}}+\omega_{s_{\mathbf{q}}}\neq 0} C^{s_{\mathbf{k}} s_{\mathbf{p}} s_{\mathbf{q}}}_{\mathbf{kpq}}\, \bar{b}^{(0)}_{s_{\mathbf{p}}}\, \bar{b}^{(0)}_{s_{\mathbf{q}}}\, e^{i(\omega_{s_{\mathbf{k}}}+\omega_{s_{\mathbf{p}}}+\omega_{s_{\mathbf{q}}})t} \,. \tag{10}$$

The sum is still over all values of the wave vectors $\mathbf{p}$ and $\mathbf{q}$ such that $\mathbf{k}+\mathbf{p}+\mathbf{q}=0$, and over the polarities $s_{\mathbf{p}} = \pm 1$, $s_{\mathbf{q}} = \pm 1$, but omitting the resonant triads, that satisfy $\omega_{s_{\mathbf{k}}} + \omega_{s_{\mathbf{p}}} + \omega_{s_{\mathbf{q}}} = 0$. The solution to this equation is:

$$b^{(1)}_{s_{\mathbf{k}}} = -\frac{i}{2} \times \sum_{\omega_{s_{\mathbf{k}}}+\omega_{s_{\mathbf{p}}}+\omega_{s_{\mathbf{q}}}\neq 0} C^{s_{\mathbf{k}} s_{\mathbf{p}} s_{\mathbf{q}}}_{\mathbf{kpq}}\, \frac{\bar{b}^{(0)}_{s_{\mathbf{p}}}\, \bar{b}^{(0)}_{s_{\mathbf{q}}}}{\omega_{s_{\mathbf{k}}}+\omega_{s_{\mathbf{p}}}+\omega_{s_{\mathbf{q}}}}\, e^{i(\omega_{s_{\mathbf{k}}}+\omega_{s_{\mathbf{p}}}+\omega_{s_{\mathbf{q}}})t} \,. \tag{11}$$

To order $\mathcal{O}(Ro^3)$, Eq. (6) yields:

$$\partial_t b^{(2)}_{s_{\mathbf{k}}} = -\partial_{T_2} b^{(0)}_{s_{\mathbf{k}}} - \partial_{T_1} b^{(1)}_{s_{\mathbf{k}}} - \nu_0 k^2 b^{(0)}_{s_{\mathbf{k}}} - \mu_0 \delta_{\mathbf{k}\cdot\hat{\mathbf{z}};0} b^{(0)}_{s_{\mathbf{k}}} + \sum C^{s_{\mathbf{k}} s_{\mathbf{p}} s_{\mathbf{q}}}_{\mathbf{kpq}}\, \bar{b}^{(0)}_{s_{\mathbf{p}}}\, \bar{b}^{(1)}_{s_{\mathbf{q}}}\, e^{i(\omega_{s_{\mathbf{k}}}+\omega_{s_{\mathbf{p}}}+\omega_{s_{\mathbf{q}}})t} \,. \tag{12}$$

We denote as $\langle\cdot\rangle$ the average over the fast time variable $t$. The left-hand side of (12) vanishes under this fast-time average, and we obtain:

$$(\partial_{T_2} + \nu_0 k^2 + \mu_0 \delta_{\mathbf{k}\cdot\hat{\mathbf{z}};0})\, b^{(0)}_{s_{\mathbf{k}}} = \sum C^{s_{\mathbf{k}} s_{\mathbf{p}} s_{\mathbf{q}}}_{\mathbf{kpq}}\, \bar{b}^{(0)}_{s_{\mathbf{p}}}(T)\, \left\langle \bar{b}^{(1)}_{s_{\mathbf{q}}}(t,T)\, e^{i(\omega_{s_{\mathbf{k}}}+\omega_{s_{\mathbf{p}}}+\omega_{s_{\mathbf{q}}})t} \right\rangle \,. \tag{13}$$

where we have used $\left\langle \partial_{T_1} b^{(1)}_{s_{\mathbf{k}}} \right\rangle = 0$. Substituting the expression of $b^{(1)}_{s_{\mathbf{k}}}$ the right-hand side becomes:

$$\sum C^{s_{\mathbf{k}} s_{\mathbf{p}} s_{\mathbf{q}}}_{\mathbf{kpq}}\, \bar{b}^{(0)}_{s_{\mathbf{p}}} \left\langle e^{i(\omega_{s_{\mathbf{k}}}+\omega_{s_{\mathbf{p}}}+\omega_{s_{\mathbf{q}}})t}\, \frac{i}{2} \sum_{\omega_{s_{\mathbf{q}}}+\omega_{s_{\mathbf{l}}}+\omega_{s_{\mathbf{r}}}\neq 0} \overline{C}^{s_{\mathbf{q}} s_{\mathbf{l}} s_{\mathbf{r}}}_{\mathbf{qlr}}\, \frac{b^{(0)}_{s_{\mathbf{l}}}\, b^{(0)}_{s_{\mathbf{r}}}}{\omega_{s_{\mathbf{q}}}+\omega_{s_{\mathbf{l}}}+\omega_{s_{\mathbf{r}}}}\, e^{-i(\omega_{s_{\mathbf{q}}}+\omega_{s_{\mathbf{l}}}+\omega_{s_{\mathbf{r}}})t} \right\rangle$$

$$= \frac{i}{2} \sum_{\omega_{s_{\mathbf{q}}}+\omega_{s_{\mathbf{l}}}+\omega_{s_{\mathbf{r}}}\neq 0} \frac{C^{s_{\mathbf{k}} s_{\mathbf{p}} s_{\mathbf{q}}}_{\mathbf{kpq}} \overline{C}^{s_{\mathbf{q}} s_{\mathbf{l}} s_{\mathbf{r}}}_{\mathbf{qlr}}}{\omega_{s_{\mathbf{q}}}+\omega_{s_{\mathbf{l}}}+\omega_{s_{\mathbf{r}}}} \bar{b}^{(0)}_{s_{\mathbf{p}}}\, b^{(0)}_{s_{\mathbf{l}}}\, b^{(0)}_{s_{\mathbf{r}}} \,, \tag{14}$$

where the latter sum is over all $\mathbf{p}$, $\mathbf{q}$, $\mathbf{l}$, $\mathbf{r}$ such that $\mathbf{p}+\mathbf{k}+\mathbf{q}=0$, $\mathbf{q}+\mathbf{l}+\mathbf{r}=0$, $\omega_{s_{\mathbf{q}}}+\omega_{s_{\mathbf{l}}}+\omega_{s_{\mathbf{r}}} \neq 0$ and $\omega_{s_{\mathbf{k}}}+\omega_{s_{\mathbf{p}}}-\omega_{s_{\mathbf{l}}}-\omega_{s_{\mathbf{r}}} = 0$, with $s_p = \pm 1$, $s_q = \pm 1$, $s_l = \pm 1$, $s_r = \pm 1$. Upon changing the blind variables $\mathbf{l}$ and $\mathbf{r}$ to $-\mathbf{l}$ and $-\mathbf{r}$, making use of the reality condition $b_s(\mathbf{k}) = \bar{b}_s(-\mathbf{k})$, we finally obtain:

$$(\partial_{T_2} + \nu_0 k^2 + \mu_0 \delta_{\mathbf{k}\cdot\hat{\mathbf{z}};0})\, b^{(0)}_{s_{\mathbf{k}}} = \frac{i}{2} \sum \frac{C^{s_{\mathbf{k}};s_{\mathbf{p}};s}_{\mathbf{k};\mathbf{p};\mathbf{l}+\mathbf{r}}\, \overline{C}^{s;s_{\mathbf{l}};s_{\mathbf{r}}}_{\mathbf{l}+\mathbf{r};-\mathbf{l};-\mathbf{r}}}{\omega_s(\mathbf{l}+\mathbf{r}) - \omega_{s_{\mathbf{l}}} - \omega_{s_{\mathbf{r}}}}\, \bar{b}^{(0)}_{s_{\mathbf{p}}}\, \bar{b}^{(0)}_{s_{\mathbf{l}}}\, \bar{b}^{(0)}_{s_{\mathbf{r}}} \,, \tag{15}$$

where the sum is over all values of $\mathbf{p}$, $\mathbf{l}$, and $\mathbf{r}$ such that $\mathbf{p}+\mathbf{k}+\mathbf{l}+\mathbf{r}=0$, $\omega_s(\mathbf{l}+\mathbf{r})-\omega_{s_{\mathbf{l}}}-\omega_{s_{\mathbf{r}}} \neq 0$, $\omega_{s_{\mathbf{k}}}+\omega_{s_{\mathbf{p}}}+\omega_{s_{\mathbf{l}}}+\omega_{s_{\mathbf{r}}} = 0$, with $s_{\mathbf{p}} = \pm 1$, $s_{\mathbf{l}} = \pm 1$, $s_{\mathbf{r}} = \pm 1$, $s = \pm 1$.

We now focus on the quartet in Fig. 4 of the Letter: the dominant flow only includes the quartet of modes we are interested in, i.e., $b^{(0)}_{s_{\mathbf{k}_2}} \neq 0$, $b^{(0)}_{s_{\mathbf{k}_3}} \neq 0$, $b^{(0)}_{s_{\mathbf{k}_4}} \neq 0$, $b^{(0)}_{s_{\mathbf{k}_5}} \neq 0$, with the polarities $(s_{\mathbf{k}_2}, s_{\mathbf{k}_3}, s_{\mathbf{k}_4}, s_{\mathbf{k}_5}) = (+1,+1,+1,-1)$, and $b^{(0)}_{s_{\mathbf{k}}} = 0$ for the other modes (except the ones needed to ensure the reality condition). Equation (15) for the mode 5 reads:

$$(\partial_{T_2} + \nu_0 k_5^2 + \mu_0)\, b^{(0)}_{s_{\mathbf{k}_5}} = C^{-1,+1,+1,+1}_{\mathbf{k}_5;\mathbf{k}_2;\mathbf{k}_3;\mathbf{k}_4}\, \bar{b}^{(0)}_{s_{\mathbf{k}_2}}\, \bar{b}^{(0)}_{s_{\mathbf{k}_3}}\, \bar{b}^{(0)}_{s_{\mathbf{k}_4}} \,, \tag{16}$$

where the quartetic interaction coefficient is:

$$\begin{aligned} C^{-1,+1,+1,+1}_{\mathbf{k}_5;\mathbf{k}_2;\mathbf{k}_3;\mathbf{k}_4} = i \Bigg[ & \frac{C^{-1;+1;+1}_{\mathbf{k}_5;\mathbf{k}_2;\mathbf{k}_3+\mathbf{k}_4}\, \overline{C}^{+1;+1;+1}_{\mathbf{k}_3+\mathbf{k}_4;-\mathbf{k}_3;-\mathbf{k}_4}}{\omega_{+1}(\mathbf{k}_3+\mathbf{k}_4) - \omega_{+1}(\mathbf{k}_3) - \omega_{+1}(\mathbf{k}_4)} + \frac{C^{-1;+1;-1}_{\mathbf{k}_5;\mathbf{k}_2;\mathbf{k}_3+\mathbf{k}_4}\, \overline{C}^{-1;+1;+1}_{\mathbf{k}_3+\mathbf{k}_4;-\mathbf{k}_3;-\mathbf{k}_4}}{\omega_{-1}(\mathbf{k}_3+\mathbf{k}_4) - \omega_{+1}(\mathbf{k}_3) - \omega_{+1}(\mathbf{k}_4)} \\ & + \frac{C^{-1;+1;+1}_{\mathbf{k}_5;\mathbf{k}_3;\mathbf{k}_2+\mathbf{k}_4}\, \overline{C}^{+1;+1;+1}_{\mathbf{k}_2+\mathbf{k}_4;-\mathbf{k}_2;-\mathbf{k}_4}}{\omega_{+1}(\mathbf{k}_2+\mathbf{k}_4) - \omega_{+1}(\mathbf{k}_2) - \omega_{+1}(\mathbf{k}_4)} + \frac{C^{-1;+1;-1}_{\mathbf{k}_5;\mathbf{k}_3;\mathbf{k}_2+\mathbf{k}_4}\, \overline{C}^{-1;+1;+1}_{\mathbf{k}_2+\mathbf{k}_4;-\mathbf{k}_2;-\mathbf{k}_4}}{\omega_{-1}(\mathbf{k}_2+\mathbf{k}_4) - \omega_{+1}(\mathbf{k}_2) - \omega_{+1}(\mathbf{k}_4)} \\ & + \frac{C^{-1;+1;-1}_{\mathbf{k}_5;\mathbf{k}_4;\mathbf{k}_2+\mathbf{k}_3}\, \overline{C}^{-1;+1;+1}_{\mathbf{k}_2+\mathbf{k}_3;-\mathbf{k}_2;-\mathbf{k}_3}}{\omega_{-1}(\mathbf{k}_2+\mathbf{k}_3) - \omega_{+1}(\mathbf{k}_2) - \omega_{+1}(\mathbf{k}_3)} \Bigg] \,. \end{aligned} \tag{17}$$

Similarly, Eq. (15) for the mode 3 reads:

$$(\partial_{T_2} + \nu_0 k_3^2)\, b^{(0)}_{s_{\mathbf{k}_3}} = C^{+1,+1,+1,-1}_{\mathbf{k}_3;\mathbf{k}_2;\mathbf{k}_4;\mathbf{k}_5}\, \bar{b}^{(0)}_{s_{\mathbf{k}_2}}\, \bar{b}^{(0)}_{s_{\mathbf{k}_3}}\, \bar{b}^{(0)}_{s_{\mathbf{k}_4}}\,, \tag{18}$$

where the quartetic interaction coefficient is:

$$C^{+1,+1,+1,-1}_{\mathbf{k}_3;\mathbf{k}_2;\mathbf{k}_4;\mathbf{k}_5} = i \left[ \frac{C^{+1;+1;-1}_{\mathbf{k}_3;\mathbf{k}_2;\mathbf{k}_5+\mathbf{k}_4} \overline{C}^{-1;-1;+1}_{\mathbf{k}_5+\mathbf{k}_4;-\mathbf{k}_5;-\mathbf{k}_4}}{\omega_{-1}(\mathbf{k}_5+\mathbf{k}_4) - \omega_{+1}(\mathbf{k}_4)} + \frac{C^{+1;-1;+1}_{\mathbf{k}_3;\mathbf{k}_5;\mathbf{k}_2+\mathbf{k}_4} \overline{C}^{+1;+1;+1}_{\mathbf{k}_2+\mathbf{k}_4;-\mathbf{k}_2;-\mathbf{k}_4}}{\omega_{+1}(\mathbf{k}_2+\mathbf{k}_4) - \omega_{+1}(\mathbf{k}_2) - \omega_{+1}(\mathbf{k}_4)} \right.$$
$$+ \frac{C^{+1;-1;-1}_{\mathbf{k}_3;\mathbf{k}_5;\mathbf{k}_2+\mathbf{k}_4} \overline{C}^{-1;+1;+1}_{\mathbf{k}_2+\mathbf{k}_4;-\mathbf{k}_2;-\mathbf{k}_4}}{\omega_{-1}(\mathbf{k}_2+\mathbf{k}_4) - \omega_{+1}(\mathbf{k}_2) - \omega_{+1}(\mathbf{k}_4)} + \frac{C^{+1;+1;+1}_{\mathbf{k}_3;\mathbf{k}_4;\mathbf{k}_2+\mathbf{k}_5} \overline{C}^{+1;+1;-1}_{\mathbf{k}_2+\mathbf{k}_5;-\mathbf{k}_2;-\mathbf{k}_5}}{\omega_{+1}(\mathbf{k}_2+\mathbf{k}_5) - \omega_{+1}(\mathbf{k}_2)}$$
$$\left. + \frac{C^{+1;+1;-1}_{\mathbf{k}_3;\mathbf{k}_4;\mathbf{k}_2+\mathbf{k}_5} \overline{C}^{-1;+1;-1}_{\mathbf{k}_2+\mathbf{k}_5;-\mathbf{k}_2;-\mathbf{k}_5}}{\omega_{-1}(\mathbf{k}_2+\mathbf{k}_5) - \omega_{+1}(\mathbf{k}_2)} \right]. \tag{19}$$

Our expressions for the quartetic interaction coefficients differ from that of SW: both polarities arise for the intermediate wavevectors of the form $\mathbf{k}_i + \mathbf{k}_j$ appearing at the denominator, provided this denominator does not vanish. Instead, SW pick the values of these polarities somewhat arbitrarily.

After substituting the expression of the triadic interaction coefficients in the expressions above, the dimensional values of the quartetic coefficients appearing in the Letter are:

$$C^{+1,+1,+1,-1}_{\mathbf{k}_3;\mathbf{k}_2;\mathbf{k}_4;\mathbf{k}_5} = \frac{k_0^2}{\Omega} \times \frac{3i}{10}(73 + 49\sqrt{5})\,, \tag{20}$$

$$C^{-1,+1,+1,+1}_{\mathbf{k}_5;\mathbf{k}_2;\mathbf{k}_3;\mathbf{k}_4} = \frac{k_0^2}{\Omega} \times \frac{24i}{5}(5 - \sqrt{5})\,, \tag{21}$$

and the product of coefficients appearing in the growth rate is:

$$C^{+1,+1,+1,-1}_{\mathbf{k}_3;\mathbf{k}_2;\mathbf{k}_4;\mathbf{k}_5} \times \overline{C}^{-1,+1,+1,+1}_{\mathbf{k}_5;\mathbf{k}_2;\mathbf{k}_3;\mathbf{k}_4} = \frac{k_0^4}{\Omega^2} \times \frac{144}{25}(30 + 43\sqrt{5}) \simeq 726\, \frac{k_0^4}{\Omega^2} > 0\,. \tag{22}$$

---

[1] L.M. Smith and F. Waleffe, Phys. Fluids **11**, 1608 (1999).
